# Supplementary material for: Improving Lagarias-Odlyzko Algorithm For Average-Case Subset Sum: Modular Arithmetic Approach
Source: arXiv:2408.16108 source file (2024-08-28)
Supplement: Supplementary file 1 [file appendix.tex]

\section{Proof of~\cref{prop:babai-inequality}}\label{sec:proof-babai-inequality}

We consider $a_1,\ldots,a_n$ to be integers drawn uniformly at random from
exponentially large range. Therefore, through the rest of this section we may
assume that $\gcd(a_1,\ldots,a_n) = 1$ as this holds with overwhelming probability.

For simplicity of the notation we denote $\Ll \coloneqq
\LO_{\textsf{tr}}(a_1,\ldots,a_n)$. LLL algorithm on lattice $\Ll$ returns the
basis of the following form:

\begin{displaymath}
\begin{pmatrix}
    \begin{matrix}
        0 & \cdots & 0
    \end{matrix}
     &\rvline& K \\
    \hline
    \makebox(1.5cm,1.5cm){$L$} & \rvline & 
    \makebox(0cm,1.5cm){$\V{v}$}
\end{pmatrix}
\end{displaymath}

for some matrix $L \in \mathbb{Z}^{(n-1) \times n}$ and vector $\V{v} \in
\mathbb{Z}^n$. Let $\V{b}_1,\ldots,\V{b}_{n-1}$ LLL-reduced basis of the matrix
$L$.

We can remark that $L$ in fact forms a basis a the lattice of vectors
which are orthogonal to $\{(a_1,\ldots,a_n)^\trans\}$. This allows us
to easily compute the determinant of this lattice, which is equal to
the norm of the vector $\{(a_1,\ldots,a_n)^\trans\}$. Thus, the
determinant is $D \coloneqq \sqrt{a_1^2+\ldots+a_n^2}$.
\antoine{We probably need a reference here.}

% Hence, the volume of $\Ll$ is equal to
% $q$. Let $a_1^{-1}$ e the inverse of $a_1$ in $\Z_q$. Because $q$ is a
% sufficiently large random number, such an inverse exists.
%
% Similarly, to the proof in~\cref{sec:Coppersmith}, observe that basis:
%
%
% \begin{displaymath}
% \begin{pmatrix}
%     1 & \alpha_2 & \alpha_3 & \cdots & \alpha_n \\
%     0 & p & 0 & & 0 \\
%     0 & 0 & p & & 0 \\
%     \vdots & \vdots &\vdots & \ddots  & \vdots \\
%     0 & 0 & 0 &\ldots & p 
% \end{pmatrix} \in \Z^{n \times n}
% \end{displaymath}
%
% \begin{displaymath}
%     \Ll^\dagger = \frac{1}{q} \left(
%     \begin{array}{cccccc}
%         a_1 & q & 0 & 0 & \cdots & 0 \\
%         a_2 & 0 & q & 0 & & 0  \\
%         a_3 & 0 & 0 & q & & 0 \\
%         \vdots & \vdots &\vdots & \ddots  & \vdots  \\
%         a_n & 0 & 0 & 0 &\ldots & q 
%     \end{array}\right),
% \end{displaymath}

Now, to complete the proof we need to somehow show a different
direction of the~\cref{lem:main-bound}:

\begin{lemma}[Proposition~\ref{prop:babai-inequality} reformulated]
    \label{lem:babai-bound}
    For every $k \in \{1,\ldots,n\}$ it holds that
    \begin{displaymath}
        \norm{\V{b}_k^\ast} \ge \gamma^{-\frac{n-1}{2}} \Vol(\Ll)^{1/n}
    \end{displaymath}
    with probability $\ge 1-2^{-\Omega(n \log{n})}$.
\end{lemma}

Note, that~\cref{lem:babai-bound} is even stronger
than~\cref{prop:babai-inequality} as it actually gives higher upper bound on
$\norm{\V{b}_k^\ast}$, because $D$ is of order $\gamma^{0.5 n^2} \cdot
\gamma^{o(n^2)}$. These $\gamma^{o(n^2)}$ are however terms of lower-order and
would offer an negligible improvement.

Analogously to our proof in~\cref{sec:coppersmith}, we will present the proof
of~\cref{lem:babai-bound} assuming the following claim.

\begin{claim} \label{event-babai}
    With $1-2^{-\Omega(n \log{n})}$ probability it holds that:
    \begin{displaymath}
        \norm{\V{b}_n^\ast} \le \Vol(\Ll)^{1/n} \le \norm{\V{b}_1^\ast}
        .
    \end{displaymath}
\end{claim}

\begin{proof}[Proof of~\cref{lem:babai-bound} assuming~\cref{event-babai}]
    Again, let us assume that both inequalities in~\cref{event-babai} hold. If
    $k \le \frac{n+1}{2}$ then by repeated application of
    inequality~\eqref{ineq:LLL3} we have that $\norm{\V{b}_k^\ast} \ge
    \gamma^{1-k} \norm{\V{b}_1^\ast} \ge \gamma^{-\frac{n-1}{2}}
    \Vol(\Ll)^{1/n}$, which is the desired result. Hence we need to focus on the
    case where $k > \frac{n+1}{2}$.

    Observe that by repeated application of inequality~\eqref{ineq:LLL3} and~\cref{event1} we have

    \begin{align*}
        \norm{\V{b}_{k+1}^\ast} \cdots \norm{\V{b}_n^\ast} &\le \prod_{i=1}^{n-k}
        \gamma^{i-1} \cdot \norm{\V{b}_n^\ast} = \gamma^{\frac{(n-k)(n-k-1)}{2}} \norm{\V{b}_n^\ast}^{n-k}
    \intertext{Similarly, we have}
        \norm{\V{b}_1^\ast} \cdots \norm{\V{b}_{k}^\ast} &\le \prod_{i=1}^{k}
        \gamma^{i-1} \norm{\V{b}_k^\ast} 
        = \gamma^{\frac{(k-1) k}{2}}
        \norm{\V{b}_k^\ast}^{k}
    \intertext{Hence by multiplying these two inequalities we have:}
        \norm{\V{b}_1^\ast} \cdots \norm{\V{b}_{n}^\ast} &\le
        \norm{\V{b}_k^\ast}^{k} \cdot \norm{\V{b}_n^\ast}^{n-k} \cdot
        \gamma^{\frac{(n-k)(n-k-1)}{2} +\frac{(k-1)k}{2}}
    \end{align*}

    Now, recall that left-hand-side is $\Vol(\Ll)$ and $\norm{\V{b}_n^\ast} \le \Vol(\Ll)^{1/n}$. Hence:

    \begin{displaymath}
        \Vol(\Ll) \le  \norm{\V{b}_k^\ast}^{k} \cdot \Vol(\Ll)^{\frac{n-k}{n}}  \cdot \gamma^{\frac{(n-k)(n-k-1)}{2} +\frac{(k-1)k}{2}}
    \end{displaymath}

    Because $k > \frac{n+1}{2}$ we have that $(n-k)(n-k-1) +(k-1)k   \le k  (n-1)$, which gives us:

    \begin{displaymath}
        \Vol(\Ll) \le \norm{\V{b}_k^\ast}^{k} \cdot \Vol(\Ll)^{\frac{n-k}{n}} \cdot 
        \gamma^{\frac{k (n-1)}{2}}
    \end{displaymath}

    By rearranging the terms we have

    \begin{displaymath}
        \gamma^{-\frac{k (n-1)}{2}} \cdot \Vol(\Ll)^{\frac{k}{n}} \le \norm{\V{b}_k^\ast}^{k} 
    \end{displaymath}

    Which after taking $k$th root gives us desired inequality.
\end{proof}

Hence, it remains to prove~\cref{event-babai}. We split the proof of this
statement into~\cref{prop:ineq1} and \cref{prop:ineq2}. First, let us prove the
left inequality.

\begin{proposition}\label{prop:ineq1}
    \begin{displaymath}
        \prob{\Vol(\Ll)^{1/n} \le \norm{\V{b}_1^\ast}} \ge 1 - 2^{-\Omega(n\log{n})}
    \end{displaymath}
\end{proposition}
\begin{proof}
    Our goal is to bound the probability that
    $\norm{\V{b}_1} \le \Vol(\Ll)^{1/n}$. Recall that $\V{b}_1 \in \Ll$.
    Hence, there exists $s_1,\ldots,s_n \in \Z$ such that:
    \begin{displaymath}
        \V{b}_1 \coloneqq \left(-\sum_{i=2}^n a_i s_i , s_2, \ldots,s_n\right)^\trans.
    \end{displaymath}
    Observe, that the number of $(s_2,\ldots,s_n)$ of length $\le \Vol(\Ll)^{1/n}$ is at most
    $\Vol(\Ball_{n-1}(D^{1/n}))$. On the other hand, because the first coordinate of
    $\V{b}_1$ is $\le D^{1/n}$, it must hold that $|\sum_{i=2}^n s_i \cdot a_i| \le D^{1/n}$.
    Recall, that $s_1,\ldots,s_n$ are randomly selected integers from the range
    $\{1,\ldots,R\}$. Therefore,
    \begin{displaymath}
        \prob{\left|\sum_{i=1}^n a_i s_i\right| \le D^{1/n}} \le 
        \sum_{i=k}^{D^{1/n}} \prob{\left(\sum_{i=1}^n a_i s_i\right) \equiv_D k}
        \le \frac{D^{1/n}}{R} \le \frac{\sqrt{n}}{D^{1-1/n}}.
    \end{displaymath}
    Finally, by the union bound we have that
    \begin{displaymath}
        \prob{\norm{\V{b}_1} < \Vol(\Ll)^{1/n}} \le \frac{\sqrt{n}}{D^{1-1/n}}
        \cdot \Vol(\Ball_{n-1}(D^{1/n})) \le 2^{-\Omega(n \log{n})}.
    \end{displaymath}

    The probability of the opposite event is at least $1 - 2^{-\Omega(n \log{n})}$.
\end{proof}

\begin{proposition}\label{prop:ineq2}
    \begin{displaymath}
        \prob{\norm{\V{b}_n^\ast} \le \Vol(\Ll)^{1/n}} \ge 1-2^{-\Omega(n \log{n})}
    \end{displaymath}
\end{proposition}
\begin{proof}
    Again recall that $\Vol(\Ll) = q$ and our goal is to bound the
    probability that $\norm{\V{b}_n^\ast} > q^{1/n}$. Now, we inspect the dual
    lattice $\Ll^\dagger$ and dual basis $\Bb^\dagger$. The dual lattice is:

    \karol{Something is wrong with the dual lattice.}

    Recall that $\norm{\V{b}_1^\dagger} \cdot \norm{\V{b}_n^\ast} = 1$. Hence we
    need to bound the probability that $\norm{\V{b}_1^\dagger} < \Vol(\Ll)^{-1/n}$.
    Now, let us inspect $\V{b}_1^\dagger$. Because $\V{b}_1^\dagger \in
    \Ll^\dagger$, in particular, by reasoning analogous to~\cref{obs:mu} we
    know that there exist integer $\kappa$ such that:

    \begin{displaymath}
        \V{b}_1^\dagger = \frac{1}{q} \cdot (\iv{\kappa a_1}_q,\ldots,\iv{\kappa a_n}_q).
    \end{displaymath}

    Moreover, note (analogously to~\cref{obs:mu}) that $\kappa$ is determined by
    the $a_1$. Hence, for a fixed $\V{y} \in \{\ceil{q/2}+1,\ldots,\floor{q/2}\}^n$ the
    congruences modulo $p$ of
    the numbers $a_2,\ldots,a_n$ are determined. This means that for a fixed $\V{y} \in \{-\ceil{q/2}+1,\ldots,\floor{q/2}\}^n$ 

    \begin{displaymath}
        \prob{\V{y} = (\iv{\kappa a_1}_p, \ldots, \iv{\kappa a_n}_p)^\trans} = \frac{1}{q^{n-1}}.
    \end{displaymath}
    
    On the other hand, the number of vectors $\V{y}$ such that
    $\norm{\frac{1}{q} \cdot \V{y}} <
    q^{1/n}$ is $\le \Vol(\Ball_n(q^{\frac{n-1}{n}}))$. Therefore by
    the union bound we have:

    \begin{displaymath}
        \prob{\norm{\V{b}_1} < q^{\frac{n-1}{n}}} <
        \frac{\Vol(\Ball_n(q^{\frac{n-1}{n}}))}{q^{n-1}} \le 2^{-\Omega(n \log{n})}.
    \end{displaymath}
\end{proof}

Both~\cref{prop:ineq1} and \cref{prop:ineq2} yield a proof
of~\cref{event-babai}, and therefore proof of~\cref{prop:babai-inequality} is
complete.
